# Supplementary material for: WonderJourney: Going from Anywhere to Everywhere
Source: arXiv:2312.03884 source file (2024-04-12)
Supplement: Supplementary file 2 [file reproducibility_statement.tex]

\section{Reproducibility Statement}\label{sec:reproduce}
To facilitate future research, we will release code upon acceptance. Note that our framework is fully modular, and the components, such as LLM, VLM, depth estimator, and outpainter, can be readily replaced by more advanced models in the future.
